# Supplementary material for: Adventures in Andromeda: The Interplay of Interstellar Dust and Gas in our Big Neighbour
Source: arXiv:2403.19798 source file (2024-03-28)
Supplement: Supplementary file 1 [file An_appendix_starform.tex]

\chapter{Cloud masks and corresponding regions in high resolution CO and \textsc{HI} maps}
\label{ap:starform}

\begin{landscape}

\end{landscape}
